# Supplementary material for: Gene Regulation by Riboswitches with and without Negative Feedback Loop
Source: arXiv:1210.6998 source file (2012-10-25)
Supplement: Supplementary file 1 [file supporting_information.pdf]

**Supporting Information for "Gene Regulation by Riboswitches with and without Negative Feedback Loop"**

**Kinetic Model:**

Here we give details of the mathematical model of riboswitch-controlled transcription with negative feedback shown schematically in Fig. 1 of the main text. The mass action rate equations corresponding to the scheme in Fig. 1 of the main text are

$$\frac{d[B]}{dt} = k_1[DNA] + k_{-f1}[B^*] - (k_{f1} + k_{t1} + \mu)[B] \quad (1)$$

$$\frac{d[B^*]}{dt} = k_{f1}[B] + k_{-b}[B^*M] - (k_{-f1} + k_b[M] + k_{t1} + \mu)[B^*] \quad (2)$$

$$\frac{d[B^*M]}{dt} = k_b[M][B^*] - (k_{-b} + k_{t1} + \mu)[B^*M] \quad (3)$$

$$\frac{d[B_2]}{dt} = k_{t1}[B] + k_{-f2}[B_2^*] - (k_{f2} + k_{t2} + \mu)[B_2] \quad (4)$$

$$\frac{d[B_2^*]}{dt} = k_{t1}[B^*] + k_{f2}[B_2] + k_{-b}[B_2^*M] - (k_{-f2} + k_b[M] + k_{t2} + \mu)[B_2^*] \quad (5)$$

$$\frac{d[B_2^*M]}{dt} = k_{t1}[B^*M] + k_b[M][B_2^*] - (k_{-b} + k_{t2} + \mu)[B_2^*M] \quad (6)$$

$$\frac{d[R_i]}{dt} = k_{t2}[B_2] - (k_{t3} + k_{d1} + \mu)[R_i] \quad (7)$$

$$\frac{d[R_f]}{dt} = k_{t3}[R_i] - (k_{d1} + \mu)[R_f[ \quad (8)$$

$$\frac{d[P]}{dt} = k_2[R_f] - (k_{d2} + \mu)[P] \quad (9)$$

$$\frac{d[M_0]}{dt} = k_3[P] + (k_{-E1} + k_{d2})[M_0E] - (k_{E1}[E] + \mu)[M_0] \quad (10)$$

$$\frac{d[M_0E]}{dt} = k_{E1}[M_0][E] - (k_{-E1} + k_{E2} + k_{d2} + \mu)[M_0E] \quad (11)$$

$$\frac{d\,[E]}{dt} = k_F\,[O_F] + (k_{-E1} + k_{E2})\,[M_0E] - (k_{E1}\,[M_0] + k_{d2} + \mu)\,[E] \quad (12)$$

$$\frac{d\,[B_{2T}]}{dt} = k_{-f2}\,[B^*_{2T}] - (k_{f2} + k_{d1} + \mu)\,[B_{2T}] \quad (13)$$

$$\frac{d\,[B^*_{2T}]}{dt} = k_{t2}\,[B^*_2] + k_{f2}\,[B_{2T}] + k_{-b}\,[B^*_{2T}M] - (k_{-f2} + k_b\,[M] + k_{d1} + \mu)\,[B^*_{2T}] \quad (14)$$

$$\frac{d\,[B^*_{2T}M]}{dt} = k_{t2}\,[B^*_2M] + k_b\,[M]\,[B^*_{2T}] - (k_{-b} + k_{d1} + \mu)\,[B^*_{2T}M] \quad (15)$$

$$\begin{aligned}\frac{d\,[M]}{dt} &= k_{E2}\,[M_0E] + k_{-b}([B^*M] + [B^*_2M] + [B^*_{2T}M]) \\ &\quad -k_b([B^*] + [B^*_2] + [B^*_{2T}])\,[M] \\ &\quad +k_{d1}\,[B^*_{2T}M] - (\mu + k_{d3})\,[M] \end{aligned} \quad (16)$$

In the model, the conversion of $M_0$ to $M$ is catalyzed by E in a two-step process: (i) $M_0$ binds to E with an association rate constant $k_{E1}$ and dissociation rate constant $k_{-E1}$. (ii) E catalyzes $M_0$ to $M$ with a catalytic rate $k_{E2}$. We choose $k_{E1} = 1$ s$^{-1}$, $k_{-E1} = 10$ s$^{-1}$, and $k_{E2} = 0.1$ s$^{-1}$ in our simulations.

Applying the model to FMN riboswitch, $M$ represents FMN, which is converted from riboflavin ($M_0$) by flavokinase ($E$). We note that FMN is subsequently converted to FAD by FAD synthetase, and riboflavin nucleotides exist *in vivo* mostly in the form of FMN and FAD, with the amount about 70%-90% in FAD. To take into account the conversion from FMN to FAD, assume the conversion rate constant is $k_{FAD}$ and the reverse rate constant is $k_{-FAD}$. The rate equations for FAD would be

$$\frac{d\,[FAD]}{dt} = k_{FAD}[M] - (k_{-FAD} + \mu)[FAD]. \quad (17)$$

There should be an additional term, $(-k_{FAD}[M] + k_{-FAD}[FAD])$, added to the rate equation for FMN (M). Assuming the conversion is fast and always in equilibrium, $d[FAD]/dt = 0$, we obtain $[FAD] = (k_{FAD}/(k_{-FAD} + \mu))[M]$. The additional term for $d[M]/dt$ becomes $-\mu\frac{k_{FAD}}{k_{-FAD}+\mu}[M]$, which is equivalent to M having an effective degradation rate of $k_{d3} = \mu\frac{k_{FAD}}{k_{-FAD}+\mu}$. Assuming 90% of flavin nucleotides are in the form FAD, and 10% in FMN, then $k_{FAD}/k_{-FAD} = 9$. Since $k_{-FAD} \gg \mu$, we then obtain $k_{d3} \sim 9\mu$ for FMN.

**Steady State Solutions:**

The steady state solutions, obtained by setting all the time derivatives to zero yield,

$$
\begin{aligned}
[B] &= \left( \frac{k_{-f1} + k_{t1} + \mu}{k_{f1}} + (\frac{k_{t1} + \mu}{k_{f1}}) \frac{[M]}{K_D} \left( 1 + \frac{k_{t1} + \mu}{k_{-b}} \right)^{-1} \right) [B^*] && (18) \\
&= K_1 \left[ 1 + \frac{k_{t1} + \mu}{k_{-f1}} \left( 1 + \frac{[M]}{K_D} \left( 1 + \frac{k_{t1} + \mu}{k_{-b}} \right)^{-1} \right) \right] [B^*] && (19) \\
&\equiv a_1(M) \, [B^*] && (20)
\end{aligned}
$$

$$
\begin{aligned}
[B^* M] &= \frac{k_b \, [M]}{k_{-b} + k_{t1} + \mu} \, [B^*] && (21) \\
&= \frac{[M]}{K_D} \left( \frac{1}{1 + \frac{k_{t1}+\mu}{k_{-b}}} \right) [B^*] && (22) \\
&\equiv a_3(M) \, [B^*] && (23)
\end{aligned}
$$

$$
\begin{aligned}
[B^*] &= \frac{k_1 \, [DNA]}{(k_{f1} + k_{t1} + \mu) a_1(M) - k_{-f1}} && (24) \\
&= \frac{k_1 \, [DNA]}{(k_{t1} + \mu) \left[ \left( 1 + \frac{[M]}{K_D} \left( 1 + \frac{k_{t1}+\mu}{k_{-b}} \right)^{-1} \right) \left( 1 + \frac{k_{t1}+\mu}{k_{f1}} \right) + K_1 \right]} && (25) \\
&\equiv \beta^*(M) \, [B'] \,, && (26)
\end{aligned}
$$

where $K_1 \equiv k_{-f1}/k_{f1}$, $K_D \equiv k_{-b}/k_b$,

$$
\begin{aligned}
[B'] &\equiv [B] + [B^*] + [B^* M] && (27) \\
&= \frac{k_1 \, [DNA]}{k_{t1} + \mu}, && (28) \\
\beta^*(M) &\equiv \left[ \left( 1 + \frac{[M]}{K_D} \left( 1 + \frac{k_{t1} + \mu}{k_{-b}} \right)^{-1} \right) \left( 1 + \frac{k_{t1} + \mu}{k_{f1}} \right) + K_1 \right]^{-1} && (29) \\
&= 1 + a_1(M) + a_3(M). && (30)
\end{aligned}
$$

From Eqs.(4),(5),(6), we obtain

$$
[B_2^*] = \frac{k_{f2} + k_{t2} + \mu}{k_{-f2}} \, [B_2] - \frac{k_{t1}}{k_{-f2}} a_1(M) \, [B^*] \qquad (31)
$$

$$
\begin{aligned}
& k_{t1}\left[1 + a_3(M)\left(\frac{1}{1+\frac{k_{t2}+\mu}{k_{-b}}}\right)\right][B^*] + k_{f2}\,[B_2] \\
& + \left[(k_{t2}+\mu)\frac{[M]}{K_D}\left(\frac{1}{1+\frac{k_{t2}+\mu}{k_{-b}}}\right) - (k_{-f2}+k_{t2}+\mu)\right][B_2^*] = 0 \qquad (32)
\end{aligned}
$$

Let

$$
c_1(M) = k_{t1}\left[1 + a_3(M)\left(\frac{1}{1+\frac{k_{t2}+\mu}{k_{-b}}}\right)\right] \qquad (33)
$$

$$
c_2(M) = (k_{t2}+\mu)\frac{[M]}{K_D}\left(\frac{1}{1+\frac{k_2+\mu}{k_{-b}}}\right) - (k_{-f2}+k_{t2}+\mu), \qquad (34)
$$

substituting Eq.(31) into Eq.(32), we obtain

$$
\begin{aligned}
[B_2] &= \frac{\frac{k_{t1}}{k_{-f2}}c_2(M)a_1(M) - c_1(M)}{k_{f2} + c_2(M)\left(\frac{k_{f2}+k_{t2}+\mu}{k_{-f2}}\right)}[B^*] \qquad (35) \\
&= \frac{c_3(M)}{c_4(M)}\left(\frac{k_{t1}}{k_{t2}+\mu}\right)[B^*] \qquad (36) \\
&= \frac{c_3(M)}{c_4(M)}\beta^*(M)\left(\frac{k_{t1}}{k_{t2}+\mu}\right)[B'] \qquad (37) \\
&= \frac{c_3(M)}{c_4(M)}\beta^*(M)\,[B_2'], \qquad (38)
\end{aligned}
$$

where

$$
\begin{aligned}
c_3(M) \equiv & -\left(\frac{k_{t2}+\mu}{k_{-f2}}\right)\frac{[M]}{K_D}\left(1+\frac{k_{t2}+\mu}{k_{-b}}\right)^{-1} a_1(M) \\
& + \left[\left(1+\frac{k_{t2}+\mu}{k_{-f2}}\right)a_1(M) + 1 + \frac{[M]}{K_D}\left(1+\frac{k_{t2}+\mu}{k_{-b}}\right)^{-1}\left(1+\frac{k_{t1}+\mu}{k_{-b}}\right)^{-1}\right] \qquad (39) \\
c_4(M) \equiv & \; 1 + \frac{1}{K_2}\left(1+\frac{[M]}{K_D}\left(1+\frac{k_{t2}+\mu}{k_{-b}}\right)^{-1}\right)\left(1+\frac{k_{t2}+\mu}{k_{f2}}\right), \qquad (40)
\end{aligned}
$$

and

$$
\begin{aligned}
[B_2'] &\equiv [B_2] + [B_2^*] + [B_2^*M] \qquad (41) \\
&= \left(\frac{k_{t1}}{k_{t2}+\mu}\right)[B']\,. \qquad (42)
\end{aligned}
$$

The steady state concentration of the fully transcribed RNA is given by

$$[R_f] \;=\; \frac{k_{t3}}{k_{t3}+k_{d1}+\mu}\,[RNA]\,, \tag{43}$$

where

$$\begin{aligned}[RNA] \;&=\; [R_i]+[R_f] \\ &=\; \frac{k_{t2}}{k_{d1}+\mu}\,[B_2]\,, \end{aligned} \tag{44}$$

and the concentration of protein P is

$$\begin{aligned}[P] \;&=\; \frac{k_2}{k_{d2}+\mu}\,[R_f] \\ &=\; \left(\frac{k_2}{k_{d2}+\mu}\right)\left(\frac{k_{t3}}{k_{t3}+k_{d1}+\mu}\right)\left(\frac{k_{t2}}{k_{d1}+\mu}\right)\frac{c_3(M)}{c_4(M)}\beta^*(M)\left(\frac{k_{t1}}{k_{t2}+\mu}\right)\left(\frac{k_1\,[DNA]}{k_{t1}+\mu}\right). \end{aligned} \tag{45}$$

From Eqs.(10),(11),(12), we can obtain

$$k_3\,[P]-(k_{E2}+\mu)\,[M_0E]-\mu\,[M_0]=0 \tag{46}$$

$$[M_0E]+[E]=\frac{k_F\,[O_F]}{\mu+k_{d2}}. \tag{47}$$

The two equations above and Eq.(11) can be further reduced to,

$$[M_0E]^2-\left[\left(\frac{k_3}{k_{E2}+\mu}\right)[P]+\left(\frac{k_F\,[O_F]}{k_{d2}+\mu}\right)+\frac{\mu}{k_{E1}(k_{E2}+\mu)}(k_{-E1}+k_{E2}+k_{d2}+\mu)\right][M_0E]$$
$$+\left(\frac{k_3}{k_{E2}+\mu}\right)[P]\left(\frac{k_F\,[O_F]}{k_{d2}+\mu}\right)=0. \tag{48}$$

The above equation is of the form

$$[M_0E]^2-b\,[M_0E]+c=0, \tag{49}$$

where $b=b(M)$ and $c=c(M)$ are functions of $[M]$. Therefore,

$$[M_0E]=\frac{b\pm\sqrt{b^2-4c}}{2}. \tag{50}$$

Let

$$x \;=\; \frac{k_F\,[O_F]}{k_{d2}+\mu} \tag{51}$$

$$y \;=\; \frac{k_3\,[P]}{k_{E2}+\mu}, \tag{52}$$

then we have $b > x + y$, and $c = xy$. It follows that

$$\sqrt{b^2 - 4c} > \sqrt{(x-y)^2} = |x - y|. \tag{53}$$

Therefore,

$$\frac{b + \sqrt{b^2 - 4c}}{2} > \frac{(x+y) + |x-y|}{2} \tag{54}$$

$$\geq x, \tag{55}$$

for any $x, y > 0$. However, from Eq.(47) and Eq.(51), we note that $x = [M_0 E] + [E]$, which means that $(b + \sqrt{b^2 - 4c})/2$ cannot be the solution for $[M_0 E]$. Hence, the only steady state solution for $[M_0 E]$ is

$$[M_0 E] = \frac{b - \sqrt{b^2 - 4c}}{2}, \tag{56}$$

which ensures $0 < [M_0 E] < x$.

From Eqs.(13),(14),(15), we obtain

$$[B_{2T}^*] = c_5(M) \left( \frac{k_{t2}}{k_{d1} + \mu} \right) \left[ [B_2^*] + [B_2^* M] \left( 1 + \frac{k_{d1} + \mu}{k_{-b}} \right)^{-1} \right], \tag{57}$$

$$[B_{2T}^* M] = \left( 1 + \frac{k_{d1} + \mu}{k_{-b}} \right)^{-1} \left( \frac{k_{t2}}{k_{-b}} [B_2^* M] + \frac{[M]}{K_D} [B_{2T}^*] \right), \tag{58}$$

where

$$c_5(M) \equiv \left[ 1 + K_2 \left( 1 + \frac{k_{d2} + \mu}{k_{f2}} \right)^{-1} + \frac{1}{K_D} \left( 1 + \frac{k_{d2} + \mu}{k_{-b}} \right)^{-1} \right]^{-1} \tag{59}$$

$$[B_2^*] = \frac{1}{K_2} \left( 1 + \frac{k_{t2} + \mu}{k_{f2}} \right) [B_2] - \frac{k_{t1}}{k_{-f2}} a_1(M) [B^*] \tag{60}$$

$$[B_2^* M] = \frac{[M]}{K_D} \left( 1 + \frac{k_{t2} + \mu}{k_{-b}} \right) \left[ \left( \frac{k_{t1}}{k_{-b} + k_{t1} + \mu} \right) [B^*] + [B_2^*] \right] \tag{61}$$

**Steady state $[M]$ production:**

By inserting Eqs.(56),(57),(58) into Eq.(15), we can get the rate of change in ligand concentration at steady state as a function of ligand concentration,

$$\frac{d[M]}{dt} = f(M). \tag{62}$$

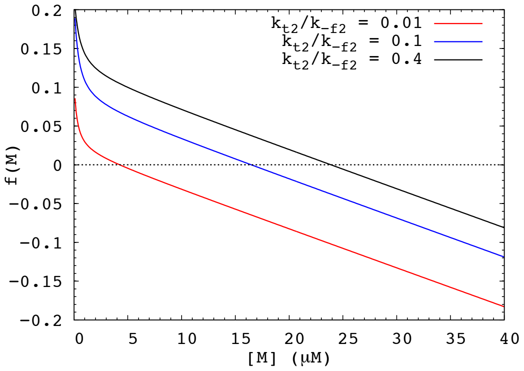


FIG. S1: Function f(M) in Eq. (60). With different parameters, $y = f(M)$ has exactly one intersect with $y = 0$, suggesting that the metaoblite concentration that makes $f(M) = 0$ is the only steady state concentration for M.

The steady state ligand concentration satisfies $f(M) = 0$. For each parameter set (Fig. S1), there is only one positive solution for the equation, and it is the only steady state. Note that in the case of $k_{t2}/k_{-f2} = 0.4$, which corresponds to the paramters from Table 1 of the main text, the steady state concentration of M is $\sim 25$ $\mu$M. This is much larger than the total concentration of RNA transcripts produced, $k_1[DNA]/(k_{d1} + \mu) \sim 14$ nM. The metabolite is in large excess over RNA transcripts, and the effective binding rate is $k_b[M] \sim 2.5$ $s^{-1}$, much faster than the RNA folding rates and transcription rates. Because of the slow dissociate rate $k_{-b} = 10^{-3}$ $s^{-1}$, all RNA transcripts with aptamer folded structures are in metabolite bound state. The riboswitch is kinetically controlled under this condition.

In the limit of $[M] = 0$, Eq.(38) becomes

$$[B_2] = \left(1 + \frac{1}{K_2}\left(1 + \frac{k_{t2} + \mu}{k_{-f2}}\right)\right)^{-1} \left[1 + \frac{\frac{k_{t2}+\mu}{k_{-f2}}\left(K_1 + \frac{k_{t1}+\mu}{k_{f1}}\right) + 1}{1 + K_1 + \frac{k_{t1}+\mu}{k_{f1}}}\right][B_2']\,. \tag{63}$$

In this limit, if $k_{t2} \ll k_{-f2}$ and $\mu \ll k_{-f2}$,

$$[B_2] \simeq \frac{K_2}{K_2 + 1}[B_2']\,, \tag{64}$$

implying the species $B_2$ and $B_2^*$ are in equilibrium. If $k_{t2} >> k_{-f2}$,

$$[B_2] \simeq \frac{K_1\left(1+\frac{k_{t1}+\mu}{k_{-f1}}\right)}{1+K_1\left(1+\frac{k_{t1}+\mu}{k_{-f1}}\right)}\,[B_2']\,. \tag{65}$$

The fraction of RNA that is not terminated early, $f_{tra} = [RNA]\,/\,[RNA]_0 = [B_2]\,/\,[B_2']$, can be expressed in terms of $K_2$ and $K_1$ in the limit of low $k_{t2}$ and high $k_{t2}$ relative to $k_{-f2}$, respectively.

As shown in Fig. 6 of the main text, the steady state concentration of protein $P$ is about 3 $\mu$M, or $\sim$ 1200 copies per cell, when using parameters from Tables 1 and 2 of the main text. If the total concentration of enzyme $E$ produced from operon $O_F$, $[E]_0 = k_F[O_F]/(\mu + k_{d2})$, is at the same level, $k_F \sim 1\ s^{-1}$ with one copy of $O_F$ per cell. Thus, we set $k_{F0} = 1\ s^{-1}$ as the reference rate for $k_F$ for the studies with feedback.
